# Supplementary material for: REST-ler: Automatic Intelligent REST API Fuzzing
Source: arXiv:1806.09739 source file (2018-06-26)
Supplement: Supplementary file 1 [file 08-appendix.tex]

\appendix

\section{Appendix}
\label{sec:appendix}

\xxx{update these graphs]}
\subsection{Complementary Graphs for \gitlab Experiments}
\begin{figure*}[t]
    \begin{minipage}{\textwidth}
    \centering
    \subfigure{
        \includegraphics[width=0.185\textwidth]{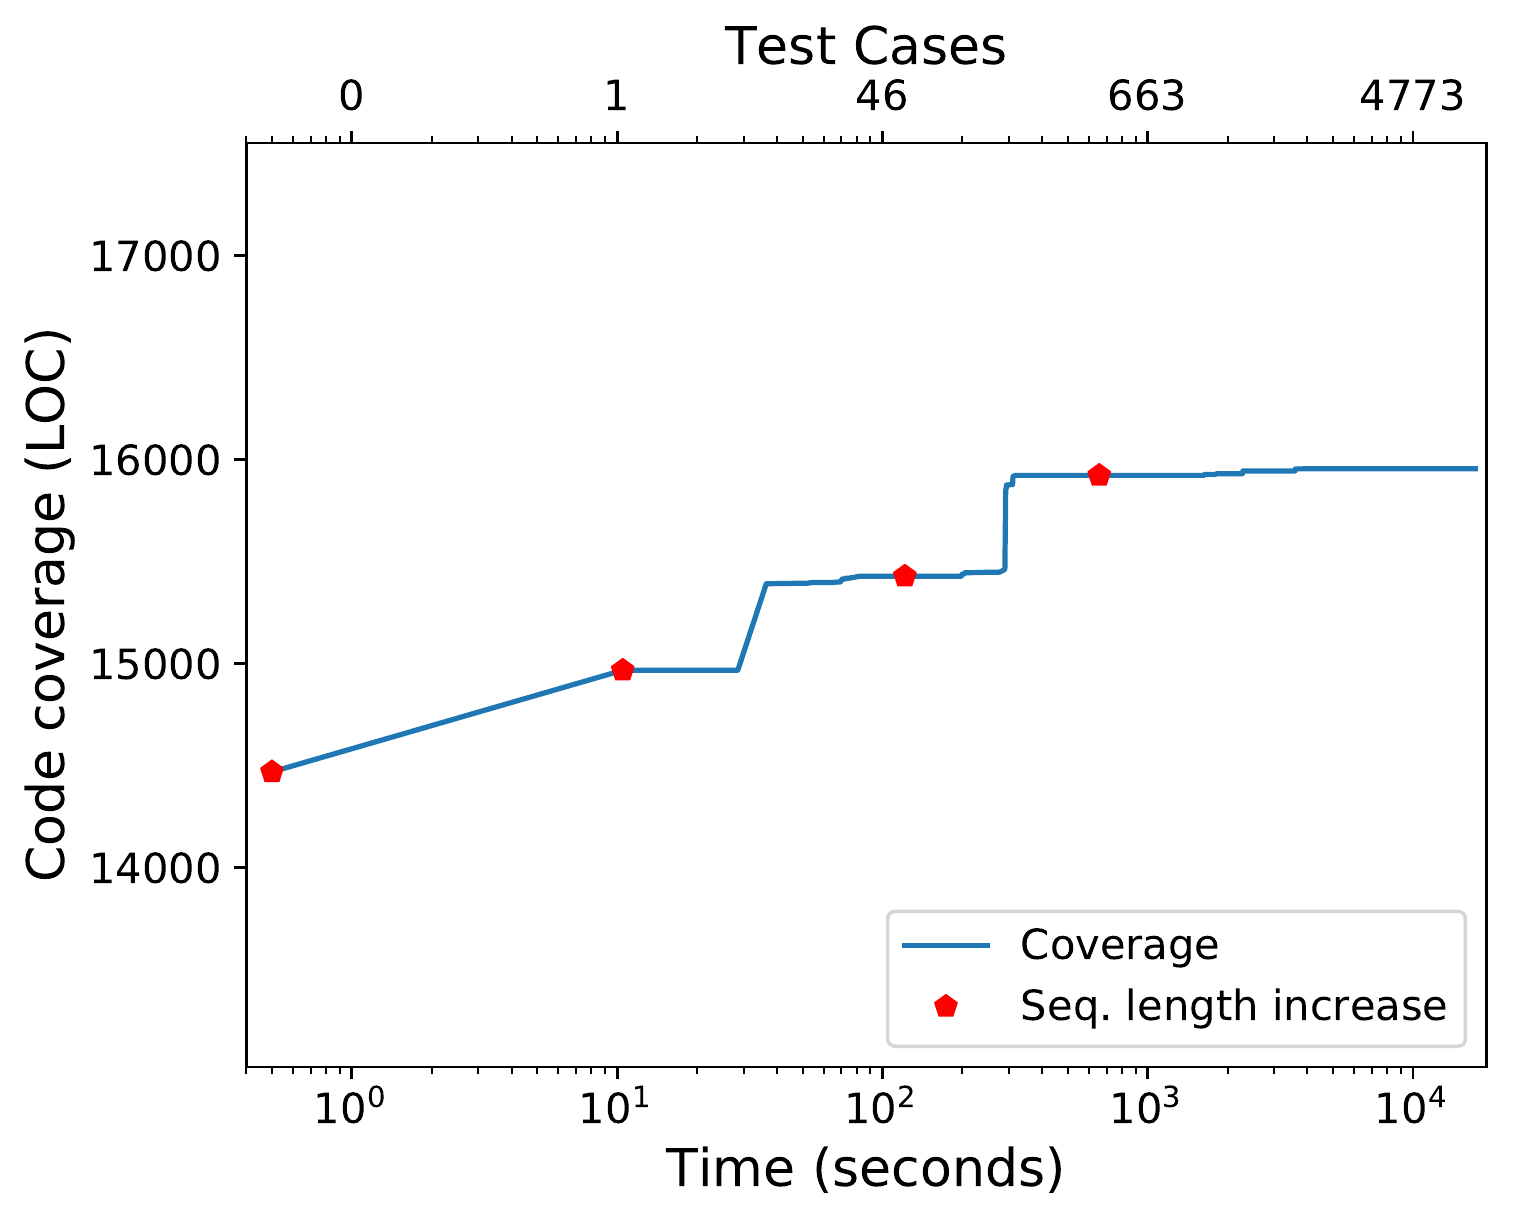}
    }
    \subfigure{
        \includegraphics[width=0.185\textwidth]{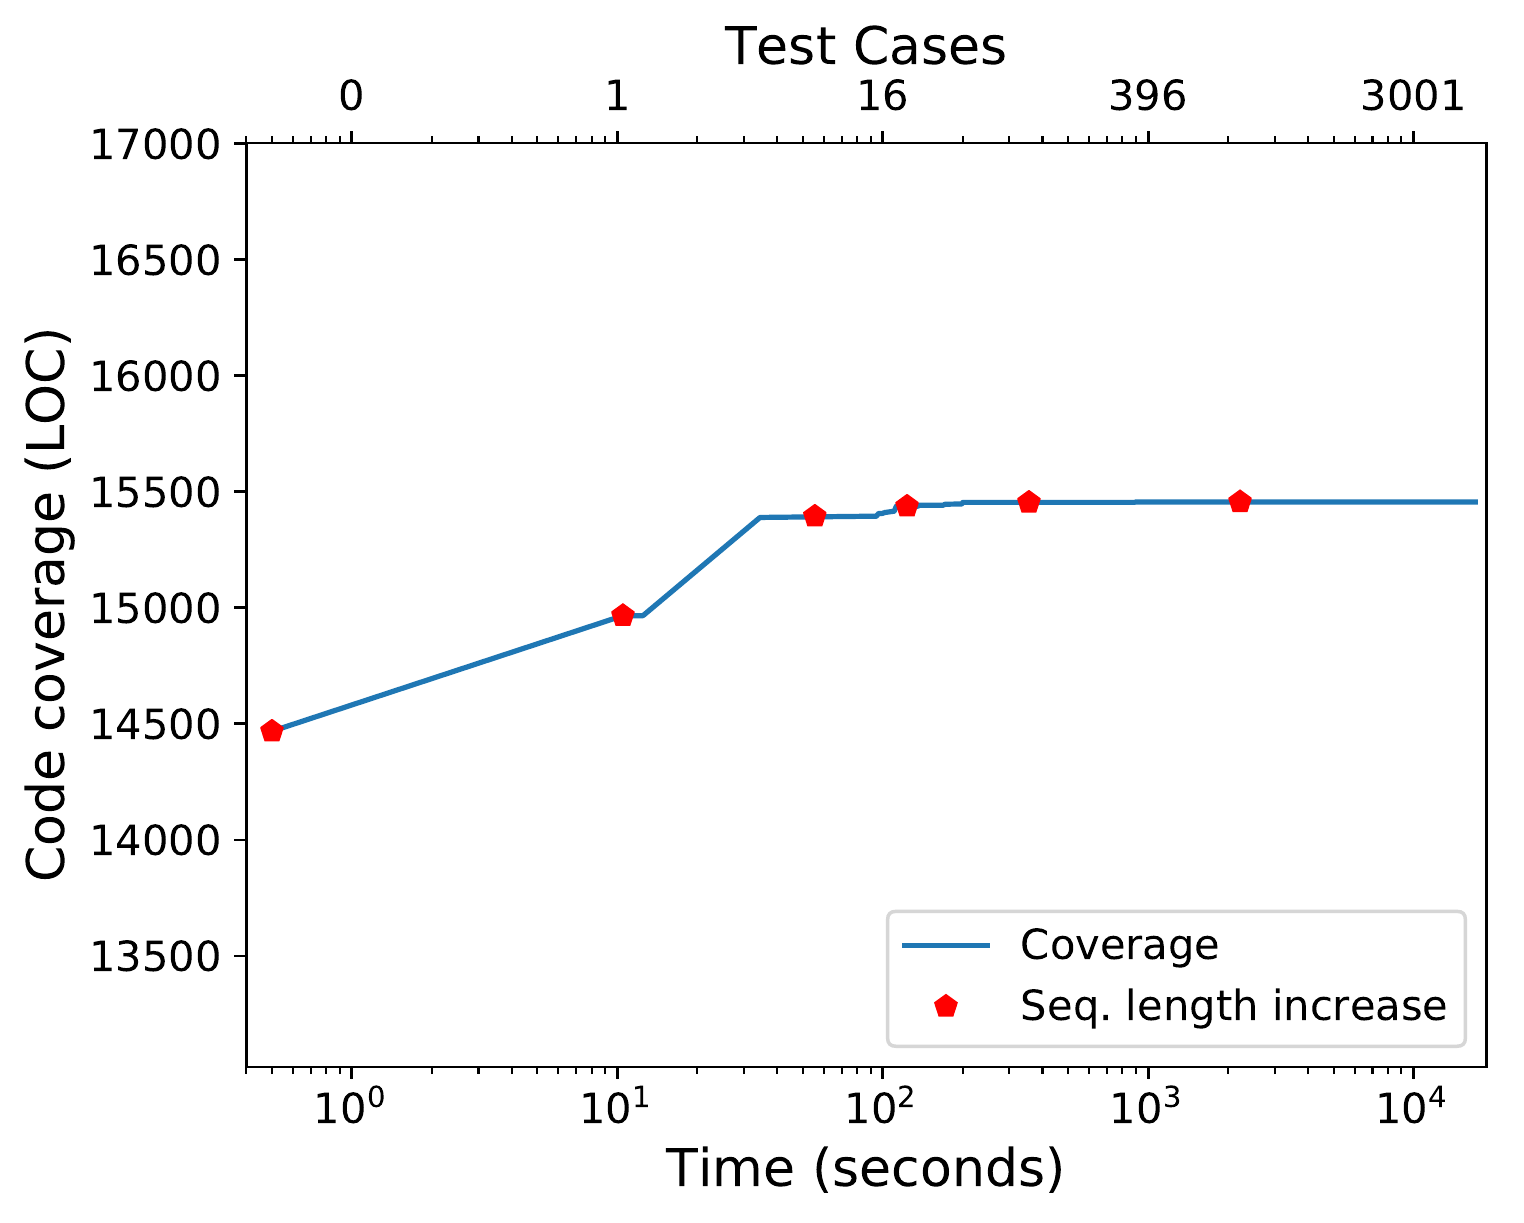}
    }
    \subfigure{
        \includegraphics[width=0.185\textwidth]{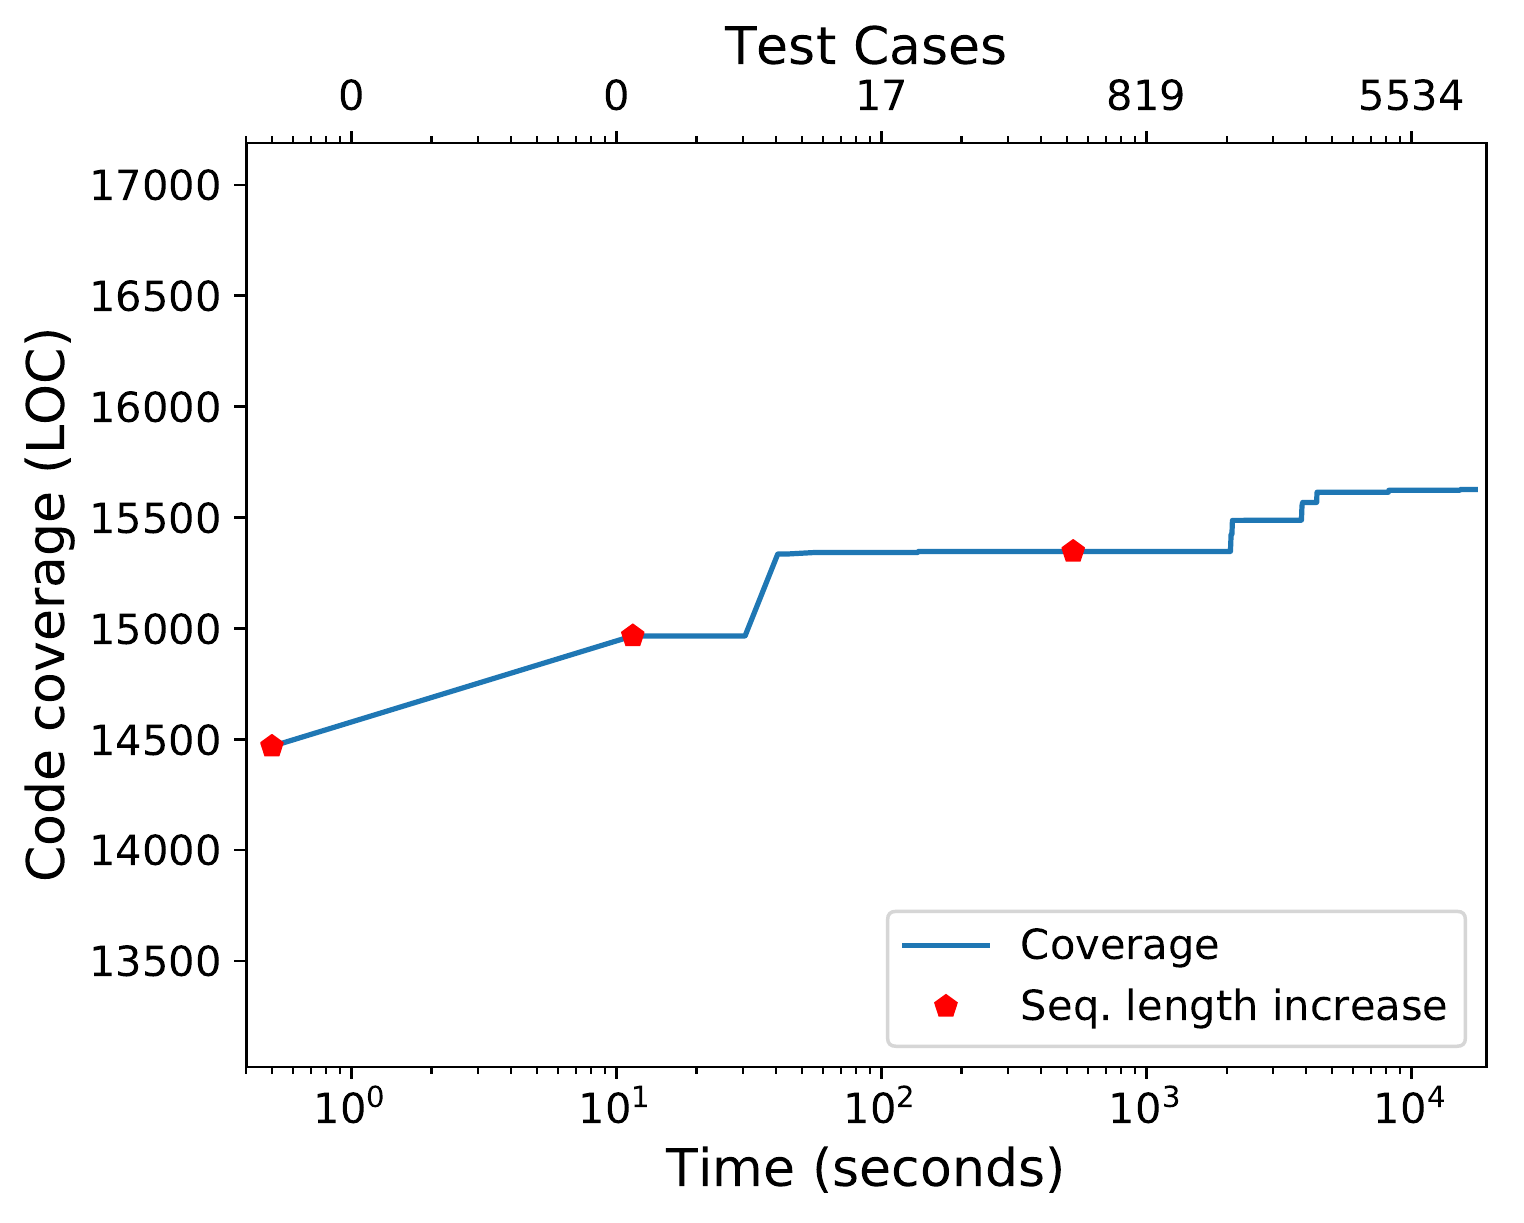}
    }
    \subfigure{
        \includegraphics[width=0.185\textwidth]{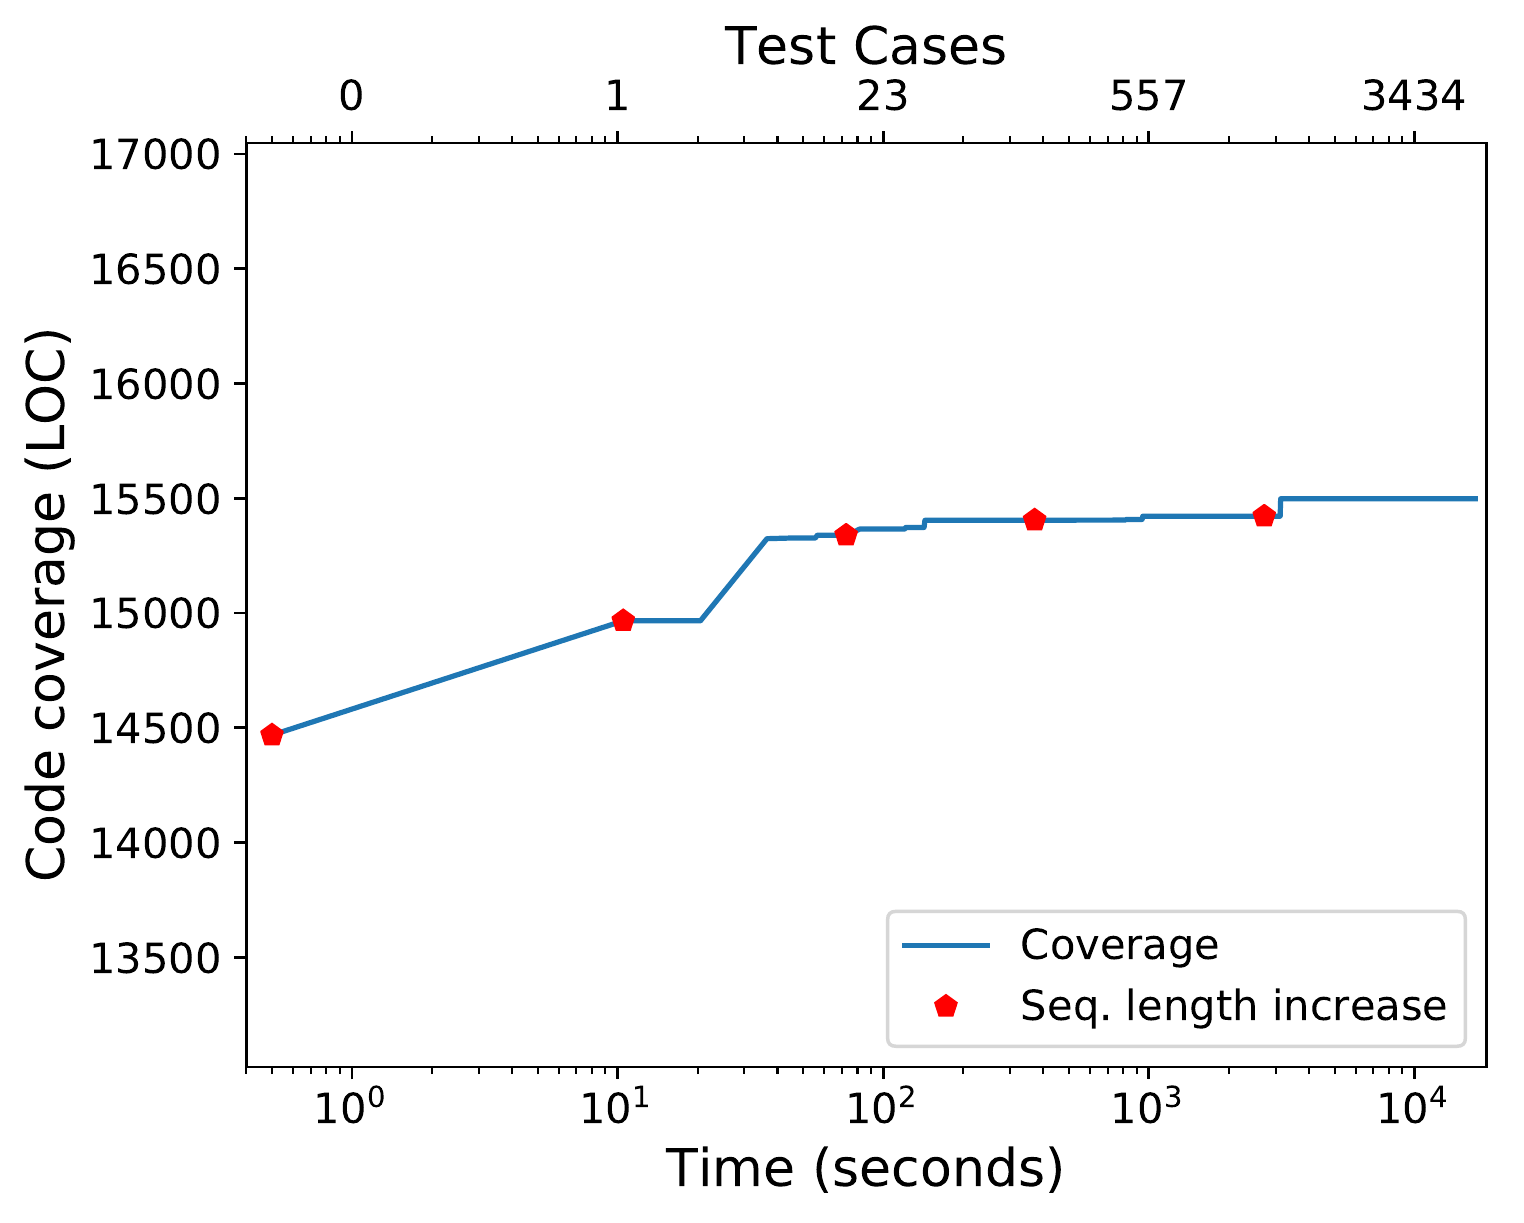}
    }
     \subfigure{
        \includegraphics[width=0.185\textwidth]{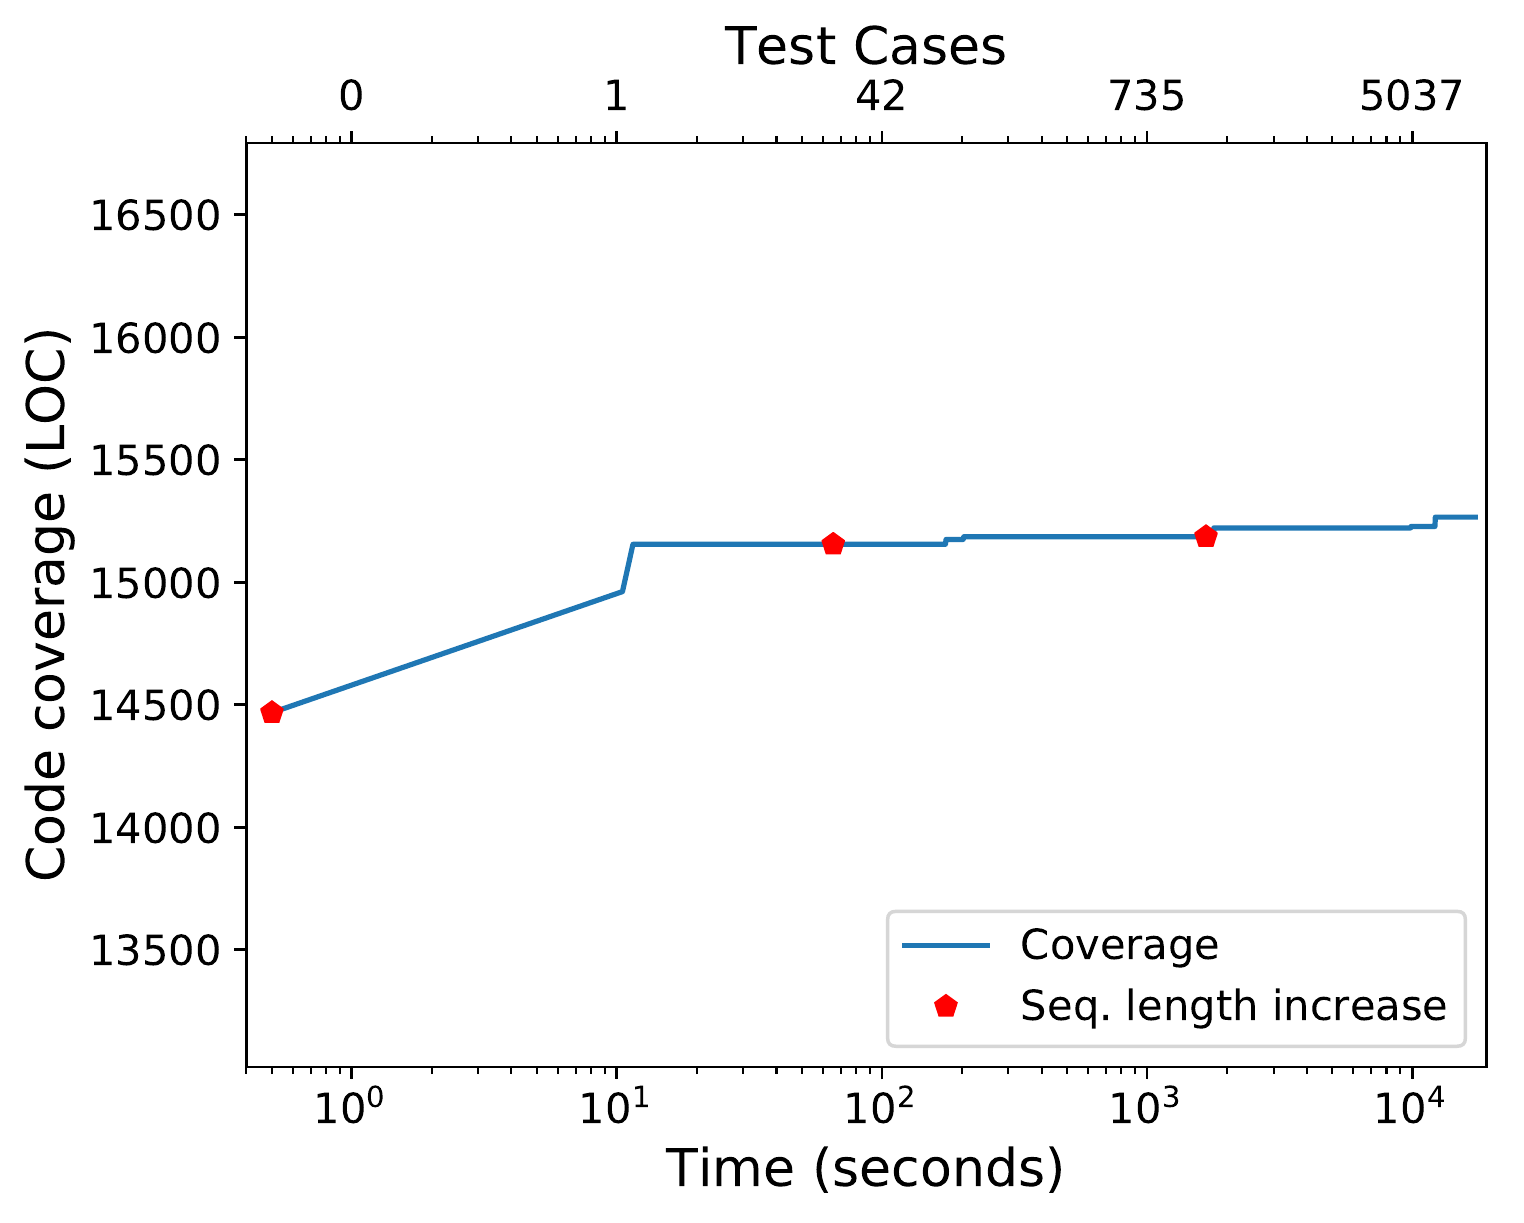}
    }
    \vspace{-8pt}
    %\caption{
    %    {\bf Code Coverage in Lines of Code Executed Over Time for \gitlab APIs.}
    %    Shows the increase in code coverage over time, while various groups of
    %    \gitlab APIs execute \restler test cases.
    %    {\underline {\em From Left to Right}} the APIs are:
    %    Commits,  Branches, Issues and Issue Notes, Repositories and Repository
    %    Files, and Groups and Members. Longer sequences capture deeper request
    %    dependencies and lead to increase in server-side code coverage.
    %}
    %\label{fig:gitlab_serverside}
    \end{minipage}\\[1em]
    \begin{minipage}{\textwidth}
    \centering
    \subfigure{
        \includegraphics[width=0.185\textwidth]{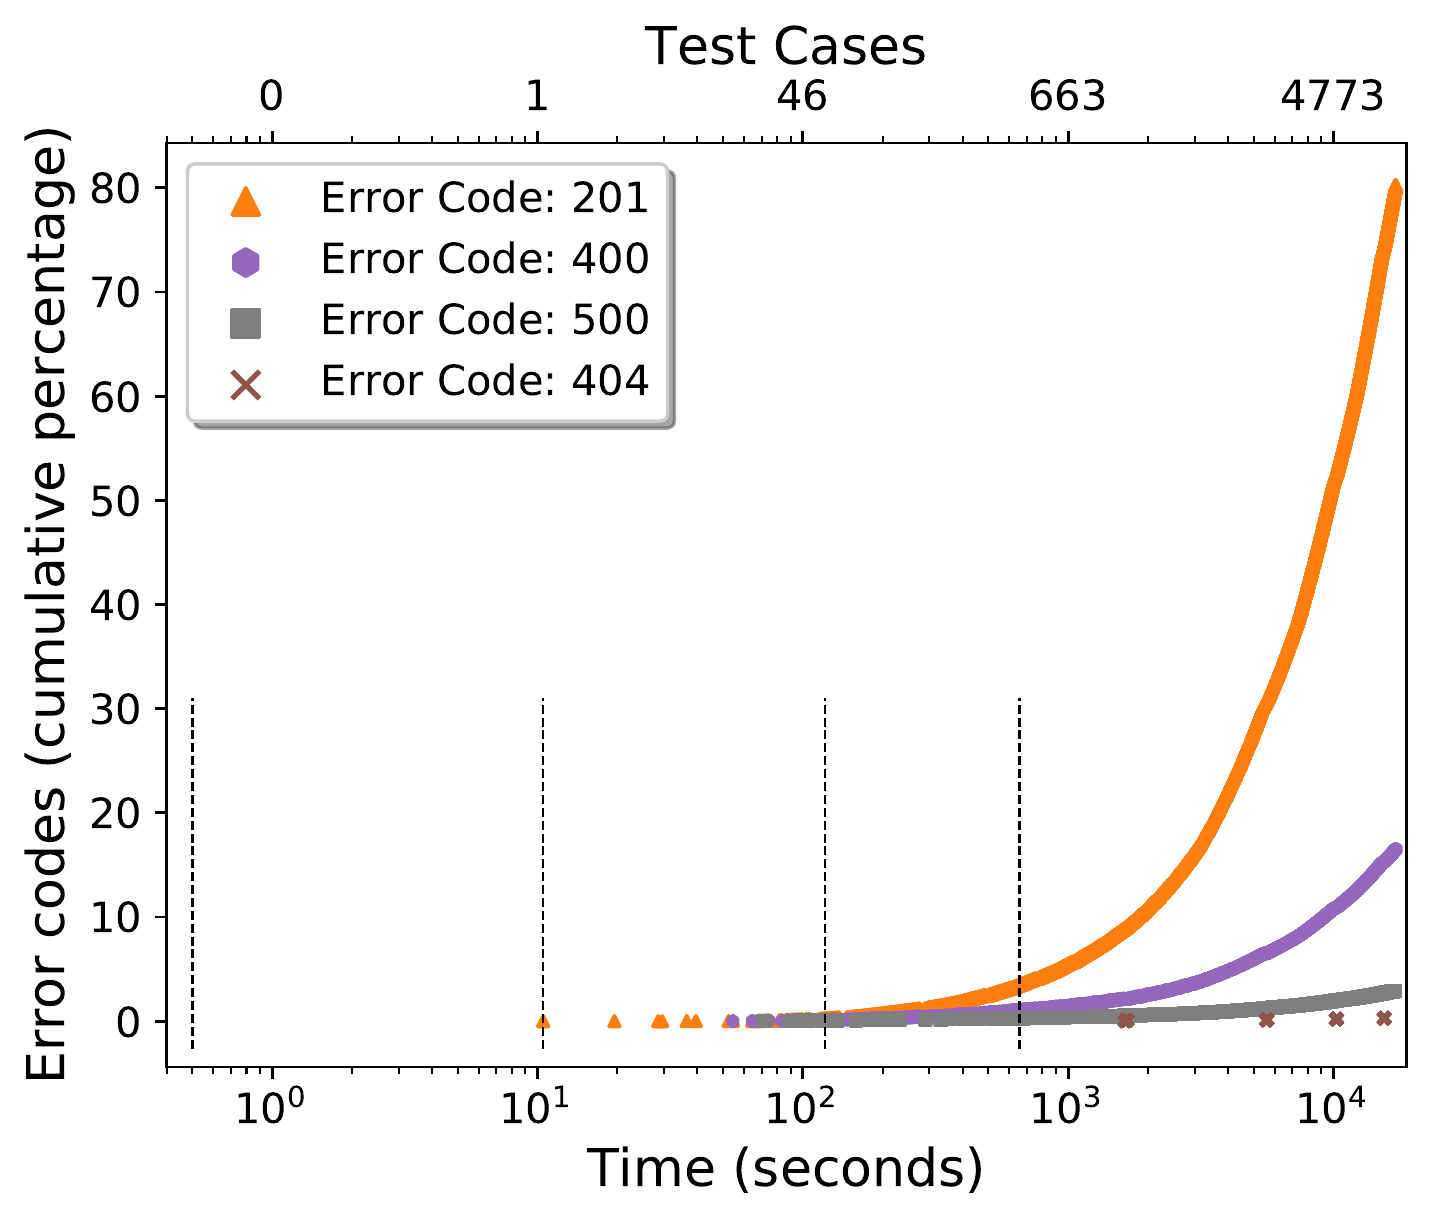}
    }
    \subfigure{
        \includegraphics[width=0.185\textwidth]{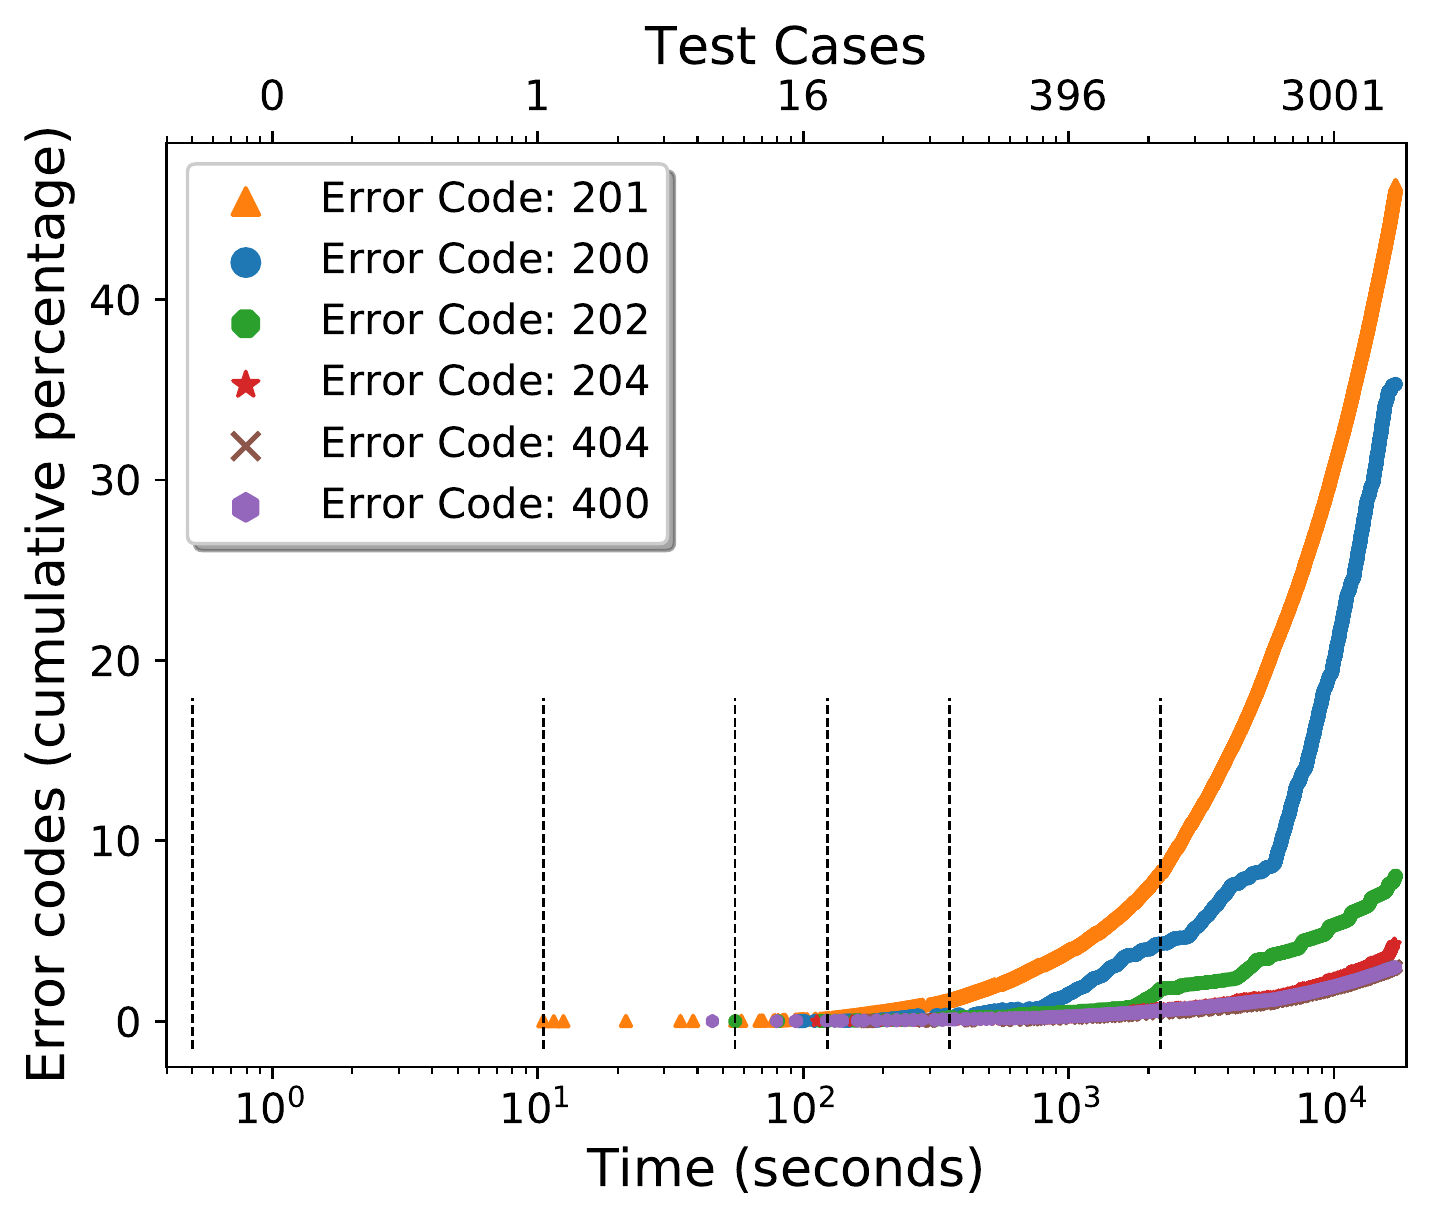}
    }
    \subfigure{
        \includegraphics[width=0.185\textwidth]{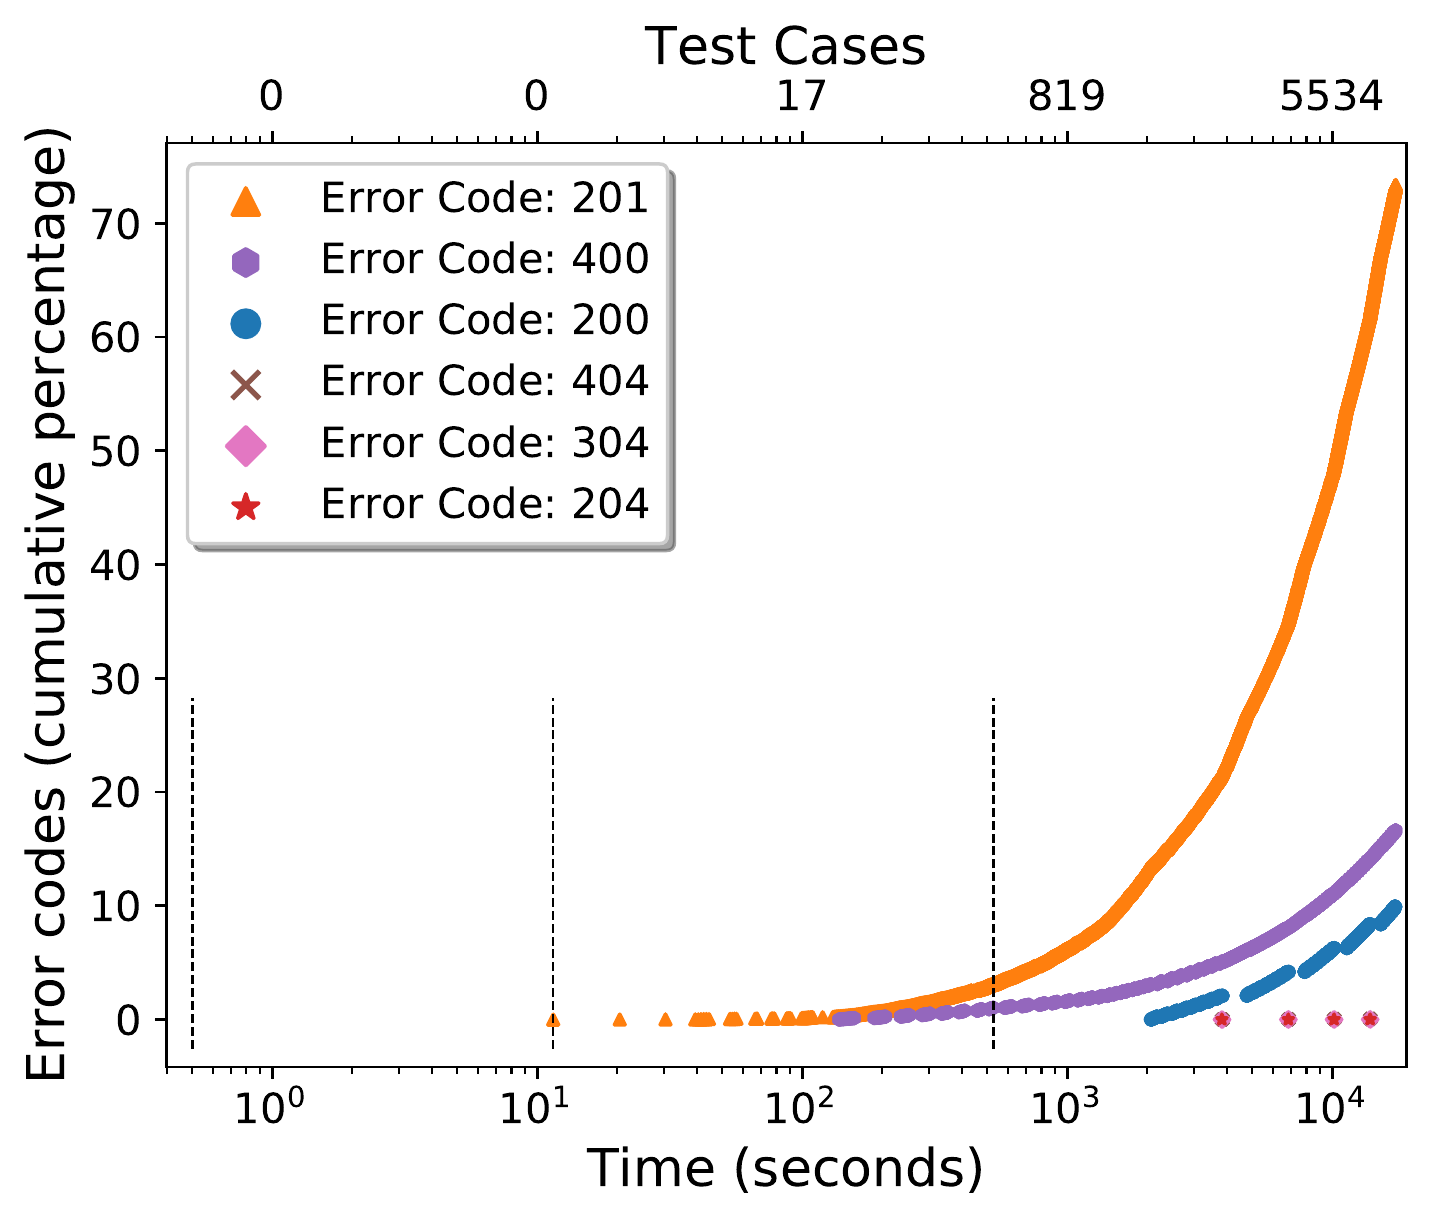}
    }
    \subfigure{
        \includegraphics[width=0.185\textwidth]{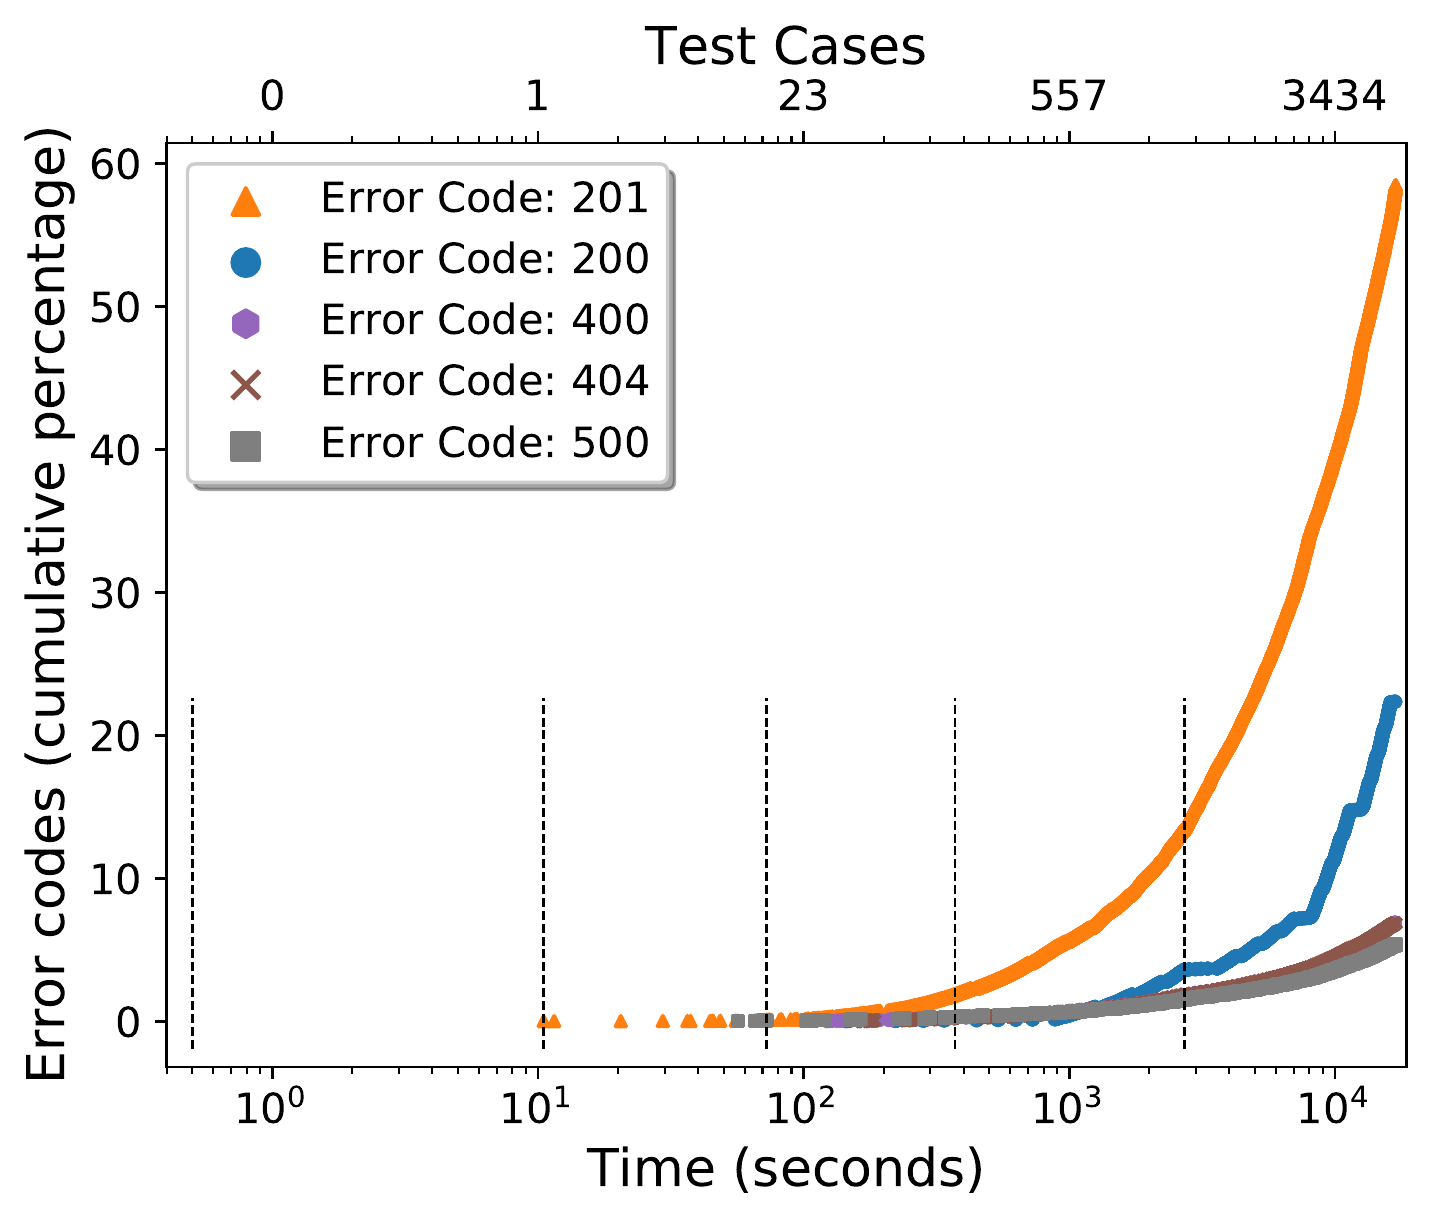}
    }
     \subfigure{
        \includegraphics[width=0.185\textwidth]{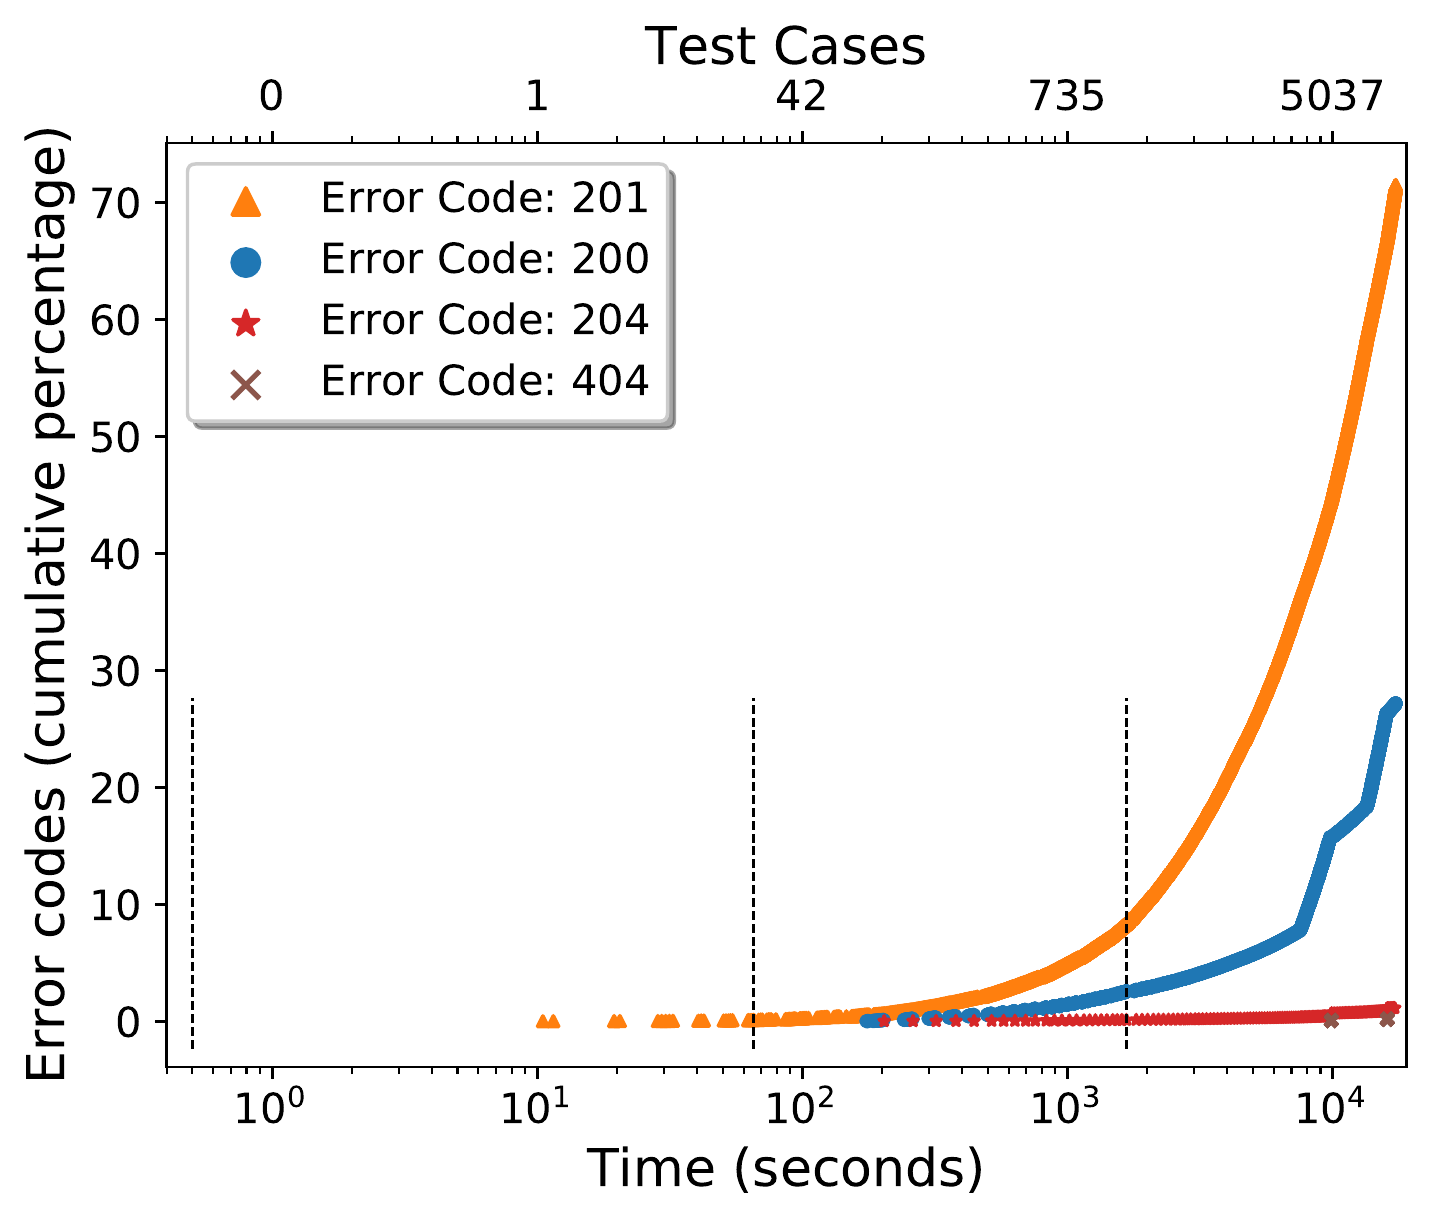}
    }
    \vspace{-10pt}
    \caption{
        {\bf Code Coverage and HTTP Status Codes Over Time for \gitlab APIs.}
        Shows the increase in code coverage (top)
        and the cumulative number or HTTP status codes received (bottom) over time,
        while various groups of \gitlab APIs execute \restler test cases.
        {\underline {\em From Left to Right}} the APIs are:
        Commits,  Branches, Issues and Issue Notes, Repositories and Repository Files,
        and Groups and Members.
        Longer sequences capture deeper dependencies of dynamic objects shared
        across
        requests and lead to increase in server-side code coverage as well as a
        variety of HTTP status codes.
    }
    \label{fig:gitlab}
   \end{minipage}
\end{figure*}
\F\ref{fig:gitlab} (top shows code coverage in lines of ruby
code, while \gitlab executes \restler test cases for various API
groups. The time is in log scale and the placement of the plots is:
Commits,  Branches,
Issues and Issue Notes, Repositories and Repository Files, and Groups and
Members (from left to right). We annotate points in time when \restler
exhausts sequences of length $N$ and moves on to sequences of length $N+1$.
Similarly, \F\ref{fig:gitlab} (bottom) shows HTTP status codes collected
over time, while \gitlab executes \restler test cases for various API groups.
The placement of the plots is the save as above.

In  top \F\ref{fig:gitlab}  we remark that increasing sequence length,
allows \restler to produce test cases that capture deeper request dependencies
and, therefore, effectively increase server-side code coverage.
Moreover, bottom \F\ref{fig:gitlab} indicates that \restler test cases trigger
a various different HTTP status codes, the vast majority of which are 20x and
40x. The prominence of these two classes of HTTP status codes is expected.
since \restler renders various primitive value commbinations (some of which
are invalid and lead to 40x HTTP status codes), and utilizes valid combinations
(which lead to 20x HTTP status codes) to compose increasingly longer sequences
of requests.

% GitLab API groups -- March 16, 2018
% -----------------------------------
% Award Emoji
% Branches
% Broadcast Messages
% Project-level Variables
% Group-level Variables
% Commits
% Custom Attributes
% Deployments
% Deploy Keys
% Environments
% Epics
% Epic Issues
% Events
% Feature flags
% Geo Nodes
% Gitignores templates
% GitLab CI Config templates
% Groups
% Group Access Requests
% Group Badges
% Group Members
% Issues
% Issue Boards
% Group Issue Boards
% Jobs
% Keys
% Labels
% License
% Merge Requests
% Merge Request Approvals
% Project milestones
% Group milestones
% Namespaces
% Notes (comments)
% Discussions (threaded comments)
% Notification settings
% Open source license templates
% Pages Domains
% Pipelines
% Pipeline Triggers
% Pipeline Schedules
% Projects including setting Webhooks
% Project Access Requests
% Project Badges
% Project import/export
% Project Members
% Project Snippets
% Protected Branches
% Repositories
% Repository Files
% Runners
% Search
% Services
% Settings
% Sidekiq metrics
% System Hooks
% Tags
% Todos
% Users
% Validate CI configuration
% V3 to V4
% Version
% Wikis
